# Supplementary material for: Simultaneous Surface Reflectance and Fluorescence Spectra Estimation
Source: arXiv:1605.04243 ancillary file (2016-05-13)
Supplement: Supplementary file 1 [file SupplementalMaterial.pdf]

# Simultaneous Surface Reflectance and Fluorescence Spectra Estimation – Supplemental Material

Henryk Blasinski, *Student Member, IEEE*, Joyce Farrell and Brian Wandell

**Abstract**—There is widespread interest in estimating the fluorescence properties of natural materials in an image. However, the separation between reflected and fluoresced components is difficult, because it is impossible to distinguish reflected and fluoresced photons only through passive observations: Separation methods require control over the illuminant spectrum. We show how to jointly estimate the reflectance and fluorescence from a single set of images acquired under multiple illuminants. We present a framework based on a linear approximation to the physical equations describing image formation in terms of surface spectral reflectance and fluorescence due to multiple fluorophores. We relax the non-convex, inverse estimation problem in order to jointly estimate the reflectance and fluorescence properties in a single optimization step and we use the Alternating Direction Method of Multipliers (ADMM) approach to efficiently find a solution. We provide a software implementation of the solver for our method and prior methods. We evaluate the accuracy and reliability of the method using both simulations and experimental data. To acquire data to test the methods, we built a custom imaging system using a monochrome camera, a filter wheel with bandpass transmissive filters and a small number of light emitting diodes. We compared the system and algorithm performance with the ground truth as well as with prior methods. Our approach produces lower errors compared to earlier algorithms.

**Index Terms**—Reflectance and Fluorescence Spectra Recovery, Multispectral and Hyperspectral Imaging, Image Color Analysis, Inverse Problems

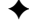

## APPENDIX A

### MULTI FLUOROPHORE ESTIMATION SOLVER

In this section we derive the Alternating Direction Method of Multipliers solver for our multi-fluorophore estimation algorithm. In order to use ADMM to solve an optimization problem it is necessary to convert the problem into a standard form, without inequality constraints. The inequality constraints can be incorporated in the objective by using set indicator functions. An equivalent problem to (16) containing equality constraints only is given as (1). The two functions  $I_{\square}$  and  $I_{\Delta}$  are set indicator functions representing constraints from the original problem. The first function, constraining the reflectance estimate to the  $[0, 1]$  interval, is defined as

$$I_{\square}(y) = \begin{cases} 0 & \text{if } 0 \leq y_i \leq 1 \ \forall i \\ \infty & \text{otherwise} \end{cases} \quad (3)$$

The second function restricts Donaldson matrix estimates to a set of matrices with nonnegative entries in their lower triangular part

$$I_{\Delta}(Y) = \begin{cases} 0 & \text{if } y_{ij} \geq 0 \ \forall j \geq i \\ \infty & \text{otherwise} \end{cases}. \quad (4)$$

ADMM is an iterative approach to solving optimization problems. In the canonical form of the ADMM algorithm, at every iteration, the augmented Lagrangian (2) is minimized first over variables  $w_r, W$ , and then over  $y_1, Y_2, Y_3$ . The scaled dual variables  $u_1, U_2, U_3$  are updated before proceeding to the next iteration. The constant in the Lagrangian represents all the terms

that are not functions of the optimization variables and therefore do not influence the minimization. Ordinarily the optimization over variables  $y_1, Y_2, Y_3$  should be conducted simultaneously. However, in this particular case the Lagrangian is separable in variables  $y_1, Y_2, Y_3$  and therefore, to simplify computations, it can be optimized over each of those variables independently. The variable update equations at iteration  $t$  are given in (5) – (11).

Note that each of the optimization steps is easy to solve. The  $w_r, W$  update consists in solving an unconstrained least-squares problem, which we perform using an iterative method; conjugate gradient algorithm initialized with the solution estimate from the previous ADMM iteration [5]. The  $y_1$  update is given by

$$y_1^{t+1} = \mathcal{P}_{\square}(B_r w_r^{t+1} + u_1^t), \quad (12)$$

where the  $\mathcal{P}_{\square}(x)$  projects every entry of  $x$  onto the interval  $[0, 1]$

$$\mathcal{P}_{\square}(x_i) = \min(\max(x_i, 0), 1). \quad (13)$$

In a similar fashion the  $Y_2$  update is given by

$$Y_2^{t+1} = \mathcal{P}_{\Delta}(B_m W^{t+1} B_x^T + U_2^t), \quad (14)$$

an operator that projects a matrix onto a set of nonnegative, lower-triangular matrices

$$\mathcal{P}_{\Delta}(y_{ij}) = \begin{cases} y_{ij} & \text{if } y_{ij} \geq 0 \ \forall i > j \\ 0 & \text{otherwise} \end{cases}. \quad (15)$$

The final update step is a nuclear norm proximal operator. Let  $W^{t+1} + U_3^t = USV^T$ , be the singular value decomposition of  $W^{t+1} + U_3^t$ , then the update operator is given by

$$Y_3^{t+1} = US_{\eta/\rho}(S)V^T. \quad (16)$$

• All authors are with the Department of Electrical Engineering, Stanford University, CA 94305. E-mail: {hblasins, jefarrell, wandell}@stanford.edu

$$\begin{aligned}
& \underset{w_r, W, y_1, Y_2, Y_3}{\text{minimize}} \quad \|M - G \circ C^T (\text{diag}(Bw_r) + T \circ B_m W B_x^T) L\|_F^2 + \alpha \|\nabla B_r w_r\|_2^2 + \\
& \quad \beta \left( \|\nabla (T \circ B_m W B_x^T)\|_F^2 + \|(T \circ B_m W B_x^T) \nabla^T\|_F^2 \right) + \\
& \quad I_{\square}(y_1) + I_{\Delta}(Y_2) + \eta \|Y_3\|_{\star} \\
& \text{subject to} \quad B_r w_r - y_1 = 0 \\
& \quad B_m W B_x^T - Y_2 = 0 \\
& \quad W - Y_3 = 0
\end{aligned} \tag{1}$$

---


$$\begin{aligned}
\mathcal{L}(w_r, W, y_1, Y_2, Y_3) = & \|M - G \circ C^T (\text{diag}(Bw_r) + T \circ B_m W B_x^T) L\|_F^2 + \alpha \|\nabla B_r w_r\|_2^2 + \\
& \beta \left( \|\nabla (T \circ B_m W B_x^T)\|_F^2 + \|(T \circ B_m W B_x^T) \nabla^T\|_F^2 \right) + I_{\square}(y_1) + I_{\Delta}(Y_2) + \eta \|Y_3\|_{\star} + \\
& \frac{\rho}{2} \left( \|B_r w_r - y_1 + u_1\|_2^2 + \|B_m W B_x^T - Y_2 + U_2\|_F^2 + \|W - Y_3 + U_3\|_F^2 \right) + \text{const}
\end{aligned} \tag{2}$$


---

$$\begin{aligned}
w_r^{t+1}, W^{t+1} = & \arg \min \|M - G \circ C^T (\text{diag}(Bw_r) + T \circ B_m W B_x^T) L\|_F^2 + \\
& \alpha \|\nabla B_r w_r\|_2^2 + \beta \left( \|\nabla (T \circ B_m W B_x^T)\|_F^2 + \|(T \circ B_m W B_x^T) \nabla^T\|_F^2 \right) + \\
& \frac{\rho}{2} \left( \|B_r w_r - y_1^t + u_1^t\|_2^2 + \|B_m W B_x^T - Y_2^t + U_2^t\|_F^2 + \|W - Y_3^t + U_3^t\|_F^2 \right)
\end{aligned} \tag{5}$$

$$y_1^{t+1} = \arg \min I_{\square}(y_1) + \frac{\rho}{2} \|B_r w_r^{t+1} - y_1^t + u_1^t\|_2^2 \tag{6}$$

$$Y_2^{t+1} = \arg \min I_{\Delta}(Y_2) + \frac{\rho}{2} \|B_m W^{t+1} B_x^T - Y_2^t + U_2^t\|_F^2 \tag{7}$$

$$Y_3^{t+1} = \arg \min \eta \|Y_3\|_{\star} + \frac{\rho}{2} \|W^{t+1} - Y_3 + U_3^t\|_F^2 \tag{8}$$

$$u_1^{t+1} = u_1^t + B_r w_r^{t+1} - y_1^{t+1} \tag{9}$$

$$U_2^{t+1} = U_2^t + B_m W^{t+1} B_x^T - Y_2^{t+1} \tag{10}$$

$$U_3^{t+1} = U_3^t + W^{t+1} - Y_3^{t+1} \tag{11}$$


---

The function  $\mathcal{S}_{\nu}(x)$  is the element-wise soft thresholding operator [3]

$$\mathcal{S}_{\nu}(x_i) = \text{sign}(x_i)(|x_i| - \nu)_+. \tag{17}$$

When the soft thresholding operator is replaced by one that selects  $n$  largest singular values the rank of the Donaldson matrix will become exactly  $n$ . This change corresponds to a non convex equality constraint  $\text{rank}(W) = n$  and consequently the ADMM algorithm may converge to a local minimum [1].

## APPENDIX B

### PARAMETER SELECTION

All algorithms we present require the user to specify a small number of parameters. These parameters describe how much emphasis, with respect to the error between measured pixel intensities and the image formation model, should be placed on spectral smoothness ( $\alpha, \beta$ ) and number of fluorophores ( $\eta$ ). For example when these parameters have high values, the optimization algorithm will prefer smooth solutions, even though they may poorly explain the captured data. For a particular imaging scenario it is necessary to select the values of these parameters to achieve the expected level of accuracy.

A grid search is a typical approach to selecting these parameters. In this approach, for every parameter, a desired number

of sample values is chosen from an interval of interest. Then the optimization is performed for all possible combinations of parameter values, and the obtained results are compared to the ground truth data. The set of parameters for which the error of the quantity of interest is lowest is typically picked.

We performed such a grid search experiment using a full camera simulation environment [2], in which the test target was composed of 24 patches having spectral reflectance of a Macbeth chart, and fluorescence excitation-emission properties of fluorophores randomly chosen from the McNamara-Boswell data set [4]. Fluorophores practical efficiency was set to 0.1. For each of the parameters 10 samples, uniformly spaced on a logarithmic, scale were chosen from the  $[10^{-3}, 10^1]$  interval. This grid search procedure produced 1000 candidate triplets for the multi-fluorophore algorithm, and 100 candidate pairs for the single fluorophore algorithm. To evaluate the performance we used the normalized root-mean-squared (RMSE) error metric.

We summarize the results of the parameter search experiment in Fig. 1 and 2 representing the multi-fluorophore and single fluorophore cases respectively. Each plot demonstrates, as a function of one parameter, the minimum error over the remaining parameters for a specified quantity of interest. Note that both algorithms are not very sensitive to the particular numerical value of the parameters, as long as their order of magnitude is reasonable.

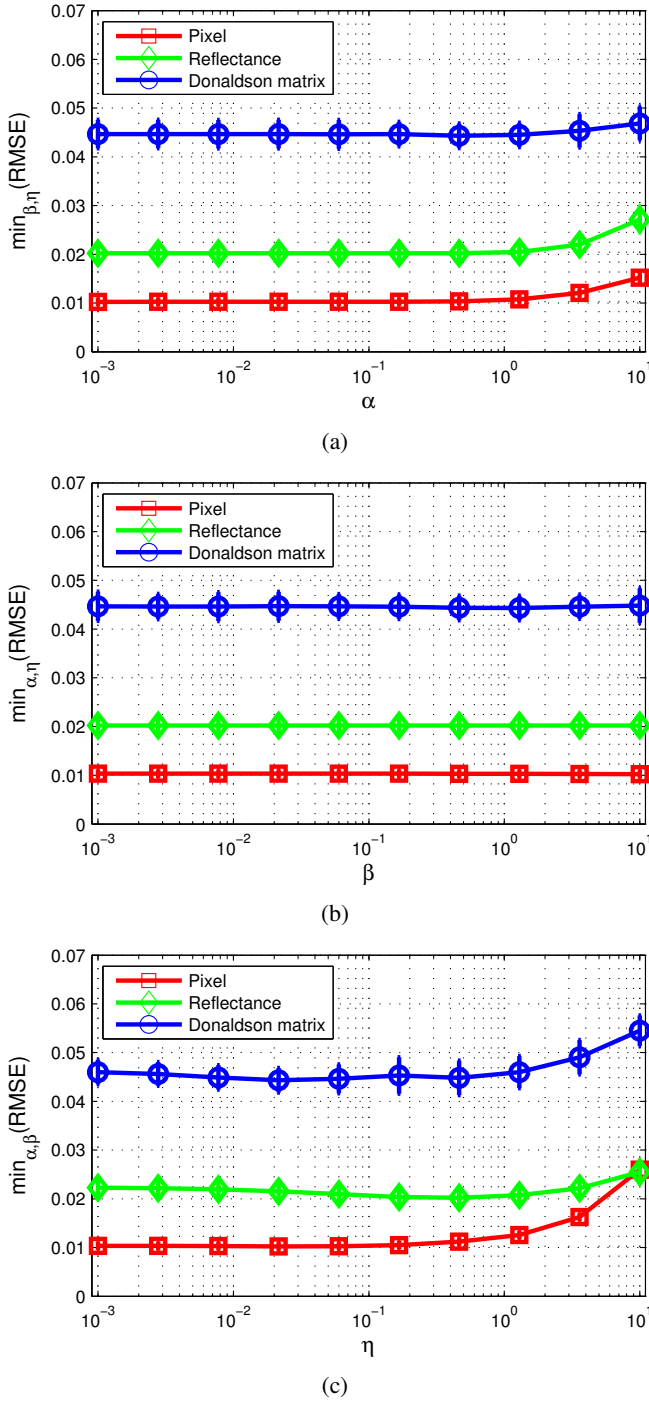

Fig. 1: Multi-fluorophore estimation error as a function of parameter values. The estimation errors remain constant over broad ranges of parameter values  $\alpha$  (a),  $\beta$  (b) and  $\eta$  (c). The curves show pixel, reflectance and normalized Donaldson matrix errors. Vertical bars represent standard error of the mean.

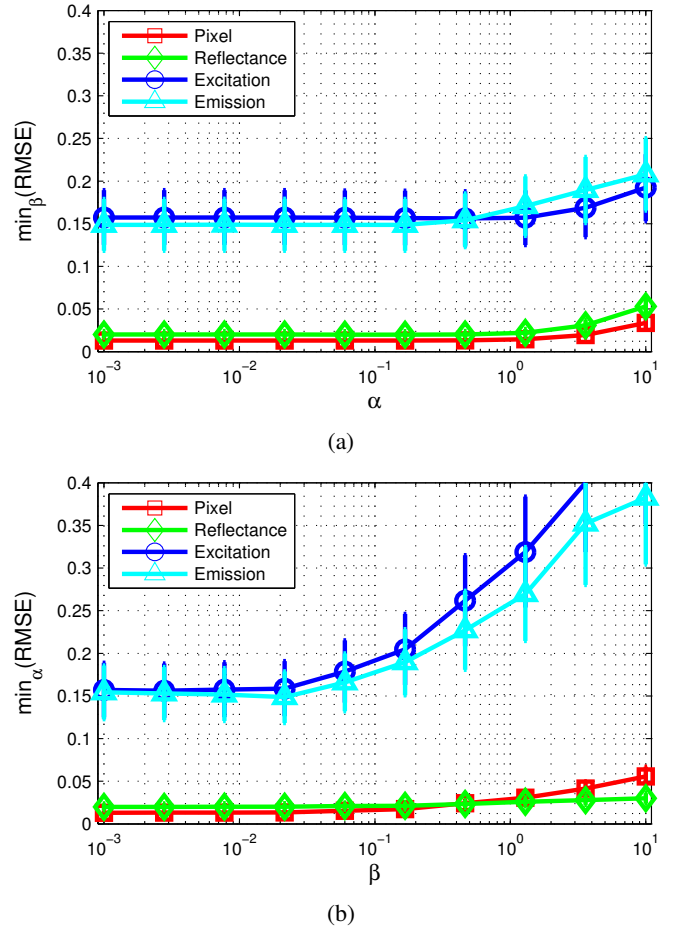

Fig. 2: Single fluorophore estimation error as a function of parameter values. The estimation errors are insensitive to small changes in  $\alpha$  (a), and  $\beta$  (b). The curves show pixel and reflectance errors as well as normalized excitation and emission spectra errors. Vertical bars represent standard error of the mean.

## APPENDIX C SIMULATION RESULTS

We used ISET toolbox [2] to validate the algorithms using full camera simulations and a variety of targets. In our simulations we used a model of the physical acquisition system we tested in experiments with physical targets. In this experiment we generated a large number of test charts with realistic reflectance and fluorescence properties. Each chart was composed of a set of Macbeth reflectances and a single fluorescent compound from the McNamara-Boswell data set [4]. This means that for a single experimental chart all Macbeth patches had identical fluorescent properties. For simulation purposes we selected about 450 fluorophores whose excitation and emission peaks were inside the 400 to 980nm spectral band. We chose this slightly narrower band, compared to the 380 to 1000nm spectral sensitivity of our device, in order to eliminate edge cases. We set fluorophores practical efficiency to 0.1. Finally, we set all the tuning parameters to  $\alpha = \beta = \eta = 0.1$ .

Figures 3 and 4 show estimation errors for each fluorophore obtained with multi- and single fluorophore algorithms respectively. For each measured quantity errors are arranged in an increasing order, but the ordering is not preserved across different quantities. For example, the test target with the 10th lowest

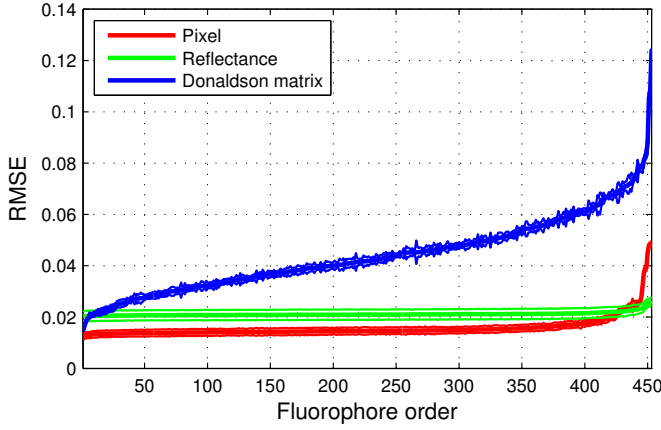

Fig. 3: Multi-fluorophore evaluation on the McNamara-Boswell dataset. Lines show the pixel prediction, reflectance and normalized Donaldson Matrix errors for different fluorophores from the McNamara-Boswell data set. For each quantity errors are sorted in the increasing order. Error bars represent the standard error over 24 patches in a test chart.

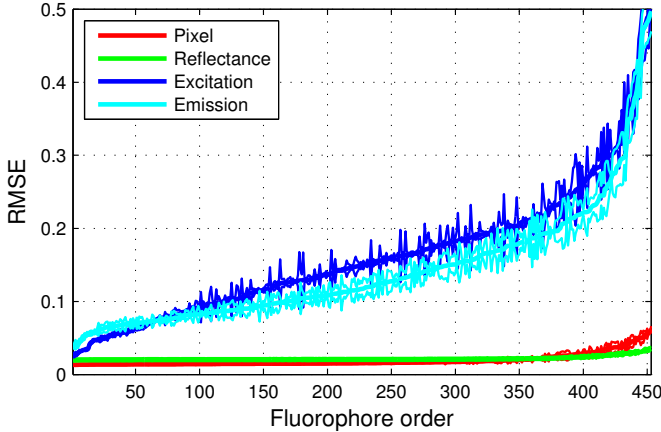

Fig. 4: Single fluorophore evaluation on the McNamara-Boswell dataset. Lines show the pixel prediction, reflectance and normalized excitation and emission errors for different fluorophores from the McNamara-Boswell data set. For each quantity errors are sorted in the increasing order. Error bars represent the standard error over 24 patches in a test chart.

reflectance error may not be the same as the target with the 10th lowest Donaldson Matrix error. Error bars represent the standard errors of the estimate computed for 24 Macbeth chart surfaces.

Observe that the predicted pixel and reflectance RMSE values are constant and independent of the fluorophore type. The Donaldson Matrix RMSE values have a larger slope, which implies some dependence between fluorophore type and estimation quality. This is understandable as fluorophores have excitation and emission peaks at different wavelengths, as well as different Stokes shifts. These properties may not be matched exactly to the illuminant spectral power distributions and/or transmissive filter locations and widths.

## APPENDIX D

### NUCLEAR NORM MINIMIZATION SOLVER

This section presents our derivation of the ADMM solver for the simultaneous reflectance and fluorescence spectra estimation method given by equation (2) in [6]. This estimation algorithm solves the optimization problem

$$\begin{aligned} & \underset{F, R, N}{\text{minimize}} \quad \|F\|_* + \alpha \|R\|_1 \\ & \text{subject to} \quad M = G \circ C^T (R + F) L + N \\ & \quad \quad \quad -3\sigma \leq N \leq 3\sigma, \end{aligned} \quad (27)$$

where  $R$  is a matrix representing surface reflectance properties, and  $F$  is the Donaldson matrix summarizing the contributions of fluorescence. Estimated quantities, represented by the three matrices  $F, R, N$  are related to the unknowns we derive in our multi-fluorophore algorithm as  $R = \text{diag}(B_r w_r)$  and  $F = B_m W B_x^T$ . The  $N$  matrix is a slack variable that limits the amount of misfit between the model and the data. Note that in the above formulation  $R$  is not restricted to being a diagonal matrix, hence the algorithm will allow nonzero off-diagonal entries. Similarly  $F$  is not limited to lower triangular matrices.

To use ADMM it is necessary to incorporate all inequality constraints directly in the objective. This leads to

$$\begin{aligned} & \underset{F, R, N}{\text{minimize}} \quad \|Y_1\|_* + \alpha \|Y_2\|_1 + I_\sigma(Y_3) \\ & \text{subject to} \quad F - Y_1 = 0 \\ & \quad \quad \quad R - Y_2 = 0 \\ & \quad \quad \quad N - Y_3 = 0 \\ & \quad \quad \quad G \circ C^T (R + F) L + N = M, \end{aligned} \quad (28)$$

where  $I_\sigma(Y)$  is an indicator function defined as

$$I_\square(Y) = \begin{cases} 0 & \text{if } -3\sigma \leq y_{ij} \leq 3\sigma \quad \forall i, j \\ \infty & \text{otherwise} \end{cases}. \quad (29)$$

The augmented Lagrangian of this problem as a function of variables  $F, R, N$  and  $Y_1, Y_2, Y_3$  is given by (18). Alternating minimization over these variables leads to update rules (19) – (26). All of the above updates are easy to compute. The  $F, R, N$  variable update requires solving an unconstrained least-squares problem. The  $Y_1$  variable update is identical to (8). The  $Y_2$  update is equivalent to applying element-wise soft thresholding to the matrix  $R^{t+1} + U_2^t$ ,

$$Y_2^{t+1} = \mathcal{S}_{\alpha/\rho}(R^{t+1} + U_2^t). \quad (30)$$

Finally, the  $Y_3$  update is given by a projection  $\mathcal{P}_\sigma$ ,

$$Y_3^{t+1} = \mathcal{P}_\sigma(N^{t+1} + U_3^t), \quad (31)$$

This projection, defined as

$$\mathcal{P}_\sigma(y) = \begin{cases} -3\sigma & \text{if } y \leq -3\sigma \\ 3\sigma & \text{if } y \geq 3\sigma \\ y & \text{otherwise} \end{cases}, \quad (32)$$

is applied to every entry of the matrix.

## REFERENCES

- [1] S. Boyd, N. Parikh, E. Chu, B. Peleato, and J. Eckstein. Distributed optimization and statistical learning via the alternating direction method of multipliers. *Foundations and Trends in Machine Learning*, 3(1):1–122, 2011.

$$\begin{aligned} \mathcal{L}(F, R, N, Y_1, Y_2, Y_3) = & \|Y_1\|_* + \alpha \|Y_2\|_1 + I_\sigma(Y_3) + \\ & \frac{\rho}{2} \left( \|F - Y_1 + U_1\|_F^2 + \|R - Y_2 + U_2\|_F^2 + \|N - Y_3 + U_3\|_F^2 + \|G \circ C^T(R + F)L + N - M + U_4\|_F^2 \right) \\ & + \text{const} \end{aligned} \quad (18)$$

$$F^{t+1}, R^{t+1}, N^{t+1} = \arg \min \|F - Y_1^t + U_1^t\|_F^2 + \|R - Y_2^t + U_2^t\|_F^2 + \|N - Y_3^t + U_3^t\|_F^2 + \|G \circ C^T(R + F)L + N - M + U_4^t\|_F^2 \quad (19)$$

$$Y_1^{t+1} = \arg \min \|Y_1\|_* + \frac{\rho}{2} \|F^{t+1} - Y_1 + U_1^t\|_F^2 \quad (20)$$

$$Y_2^{t+1} = \arg \min \alpha \|Y_2\|_1 + \frac{\rho}{2} \|R^{t+1} - Y_2 + U_2^t\|_F^2 \quad (21)$$

$$Y_3^{t+1} = \arg \min I_\sigma(Y_3) + \frac{\rho}{2} \|N^{t+1} - Y_3 + U_3^t\|_F^2 \quad (22)$$

$$U_1^{t+1} = U_1^t + F^{t+1} - Y_1^{t+1} \quad (23)$$

$$U_2^{t+1} = U_2^t + R^{t+1} - Y_2^{t+1} \quad (24)$$

$$U_3^{t+1} = U_3^t + N^{t+1} - Y_3^{t+1} \quad (25)$$

$$U_4^{t+1} = U_4^t + G \circ C^T(R^{t+1} + F^{t+1})L + N^{t+1} - M \quad (26)$$

- [2] J. E. Farrell, F. Xiao, P. B. Catrysse, and B. A. Wandell. A simulation tool for evaluating digital camera image quality. In *Electronic Imaging*, pages 124–131. International Society for Optics and Photonics, 2003.
- [3] T. Hastie, R. Tibshirani, and J. Friedman. *The Elements of Statistical Learning*. Springer, 2001.
- [4] G. McNamara, A. Gupta, J. Reynaert, T. D. Coates, and C. Boswell. Spectral imaging microscopy web sites and data. *Cytometry*, 69A(8):863–871, 2006.
- [5] J. Nocedal and S. J. Wright. *Numerical Optimization*. Springer, 2006.
- [6] J. Suo, L. Bian, F. Chen, and Q. Dai. Bispectral coding: compressive and high-quality acquisition of fluorescence and reflectance. *Optics Express*, 22(2):1697–1712, Jan 2014.
